# Supplementary material for: Magnetization reversal and domain structures in perpendicular synthetic antiferromagnets prepared on rigid and flexible substrates
Source: arXiv:2203.02733 source file (2022-03-05)
Supplement: Supplementary file 1 [file Supplementary_Bedanta.pdf]

# Supplementary Information

## Magnetization reversal and domain structures in perpendicular synthetic antiferromagnets prepared on rigid and flexible substrates

Shaktiranjan Mohanty[1], Minaxi Sharma[1], Ashish K. Moharana[1], Brindaban Ojha[1], Esita Pandey[1], Braj Bhusan Singh[1], and Subhankar Bedanta[1,2]

[1] Laboratory for Nanomagnetism and Magnetic Materials (LNMM), School of Physical Sciences, National Institute of Science Education and Research (NISER), An OCC of Homi Bhabha National Institute (HBNI), Jatni 752050, Odisha, India

[2] Center for Interdisciplinary Sciences(CIS), National Institute of Science Education and Research (NISER), An OCC of Homi Bhabha National Institute (HBNI), Jatni 752050, Odisha, India

sbedanta@niser.ac.in

The hysteresis loops of samples R1 and S1 – S8 are shown in figures S1 and S2, respectively, measured by SQUID-VSM in which the field was applied in the out-of-plane configuration. The reference sample R1 clearly shows a perpendicular magnetic anisotropic (PMA) behaviour.

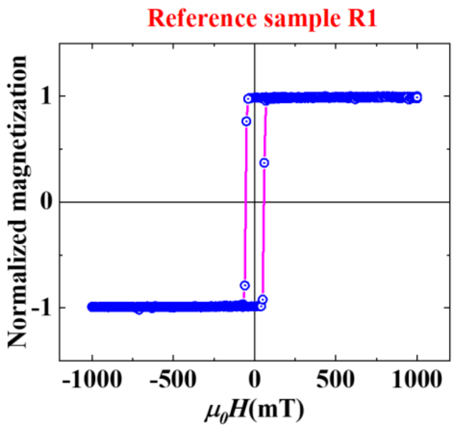


Figure S1: Hysteresis loop measured by SQUID-VSM for the reference sample R1 without Ir spacer.

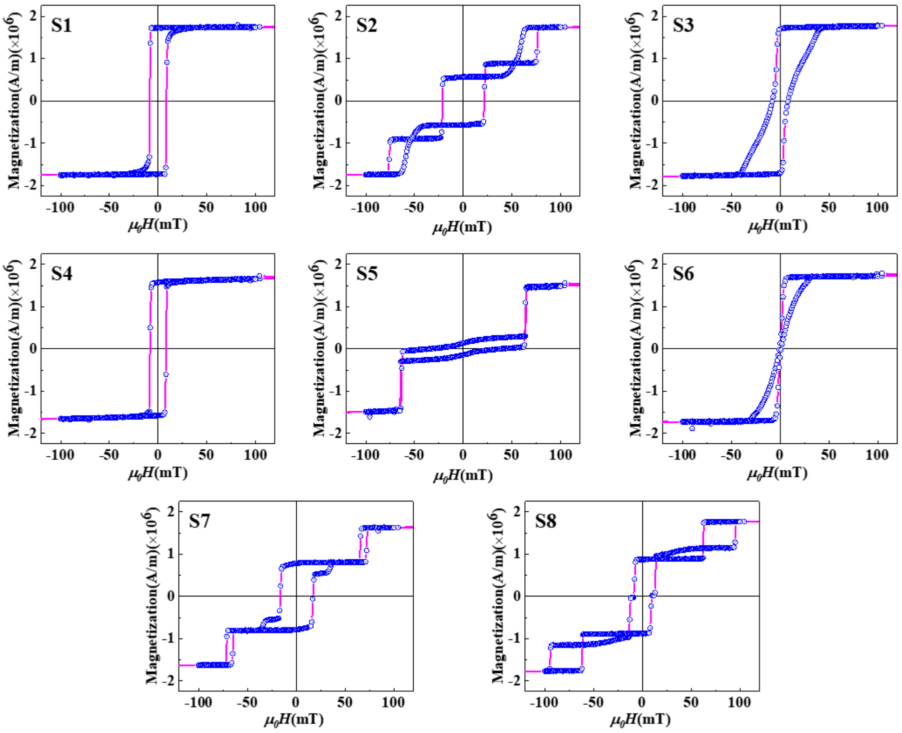

Figure S2: Hysteresis loop of samples S1-S8 measured by SQUID-VSM in which the field was applied in the out-of-plane configuration.

Figure S3 (a) shows the hysteresis loop of sample S1 and (b), (c), (d) and (e) show the corresponding domain images of respective points shown in the hysteresis loop (a). Similarly, Fig. S3 (b) shows the hysteresis loop of sample S4 and (g), (h), (i) and (j) show the corresponding domain images of respective points shown in the hysteresis loop (f).

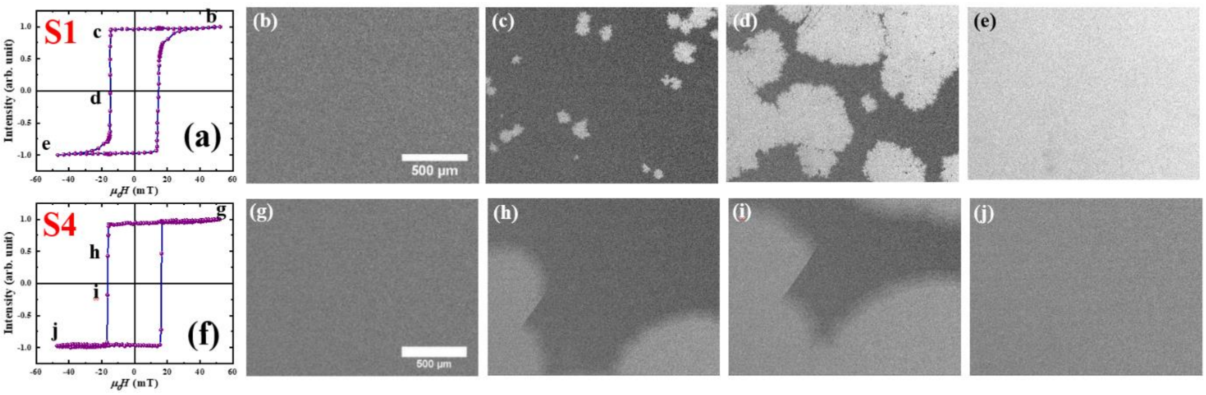

FigureS3: Hysteresis loops and corresponding domain images of samples S1 and S4

In order to evaluate the thicknesses of the layers, we have performed x-ray reflectivity using a x-ray diffractometer manufactured by Rigaku, Japan. From the XRR fitting, the following parameters are found for sample S5 which are listed in the table S1. The parameters found from the XRR fit almost matches the expected thickness we deposited using the QCM calibration. The XRR fit is shown in Fig. S4.

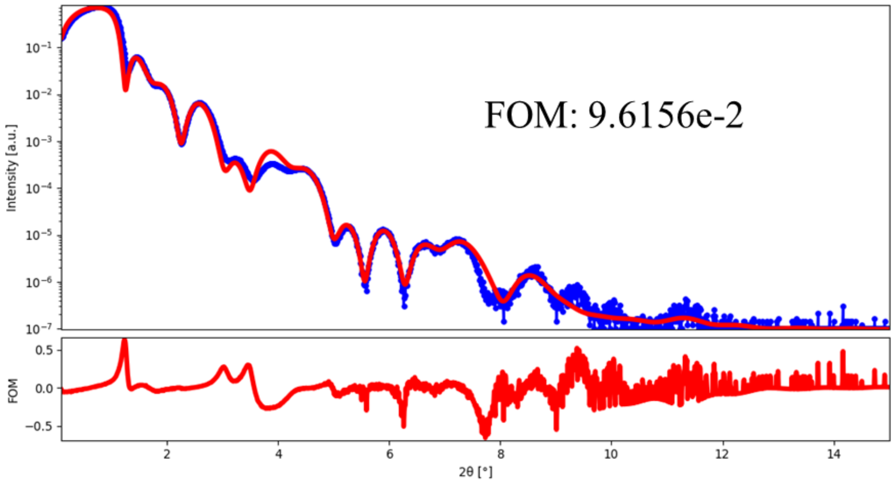


Figure S4: XRR data and best fits for the sample S5.

Table S1: XRR fit parameters for sample S5.

| Material | Thickness(in nm) | Roughness(in nm) |
|---|---|---|
| Ta | 3.36 | 0.36 |
| Pt | 2.99 | 1.4 |
| Co | 0.84 | 0.2 |
| Ir | 1.49 | 0.31 |
| Co | 0.81 | 0.29 |
| Pt | 3.31 | 0.41 |

The area between Ms and the in-plane *M–H* curves represents the effective anisotropy ($K_{eff}$) of a system. So the $K_{eff}$ can be written as, $K_{eff} = (1/2)\mu_0 H_s M_s$. Here *Hs* is the intersecting point of saturation field of in-plane and out-of-plane hysteresis loops (shown in figure S5) and Ms is saturation magnetization.

Table S2: Anisotropy energy calculation for all the samples from the SQUID data.

| Sample name | Saturation Magnetization(M*s*) in A/m | Anisotropy field($H_k$) in mT | Anisotropy energy($K_{eff}$) in *J/m*3 |
|---|---|---|---|
| S1 | $1.75\times10^{6}$ | 969 | $8.47\times10^{5}$ |
| S2 | $1.75\times10^{6}$ | 1100 | $9.62\times10^{5}$ |
| S3 | $1.78\times10^{6}$ | 837 | $7.44\times10^{5}$ |
| S4 | $1.74\times10^{6}$ | 781 | $6.79\times10^{5}$ |
| S5 | $1.59\times10^{6}$ | 1138 | $9.04\times10^{5}$ |
| S6 | $1.76\times10^{6}$ | 631 | $5.55\times10^{5}$ |
| S7 | $1.64\times10^{6}$ | 1183 | $9.70\times10^{5}$ |
| S8 | $1.78\times10^{6}$ | 1302 | $1.15\times10^{6}$ |

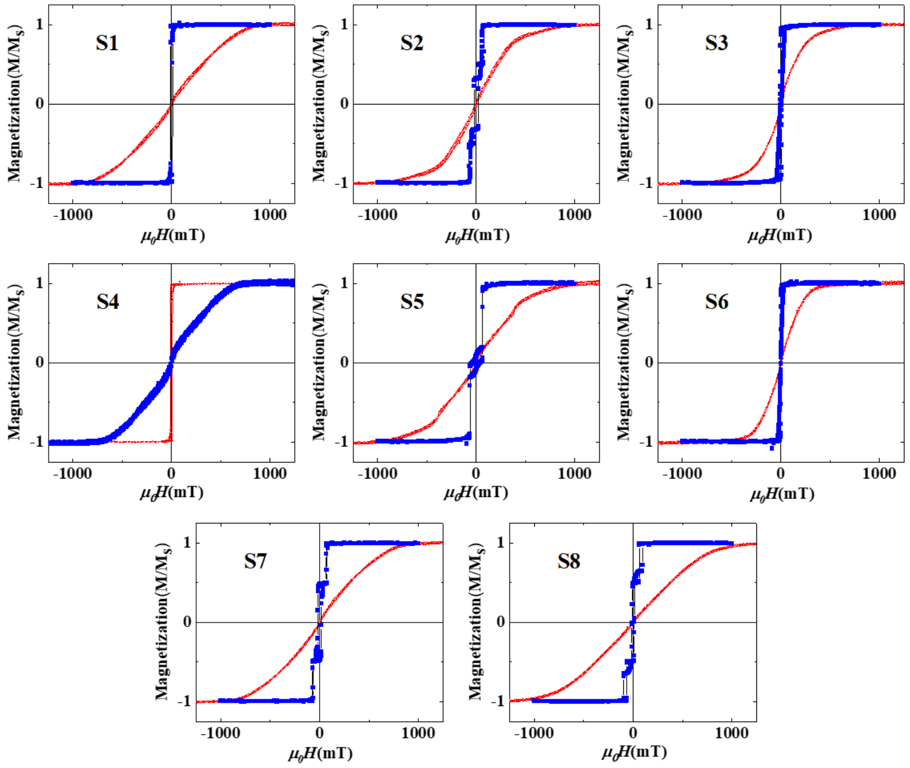


Figure S5: In-plane and out-of-plane hysteresis loop of samples S1 to S8 measured via SQUID VSM.

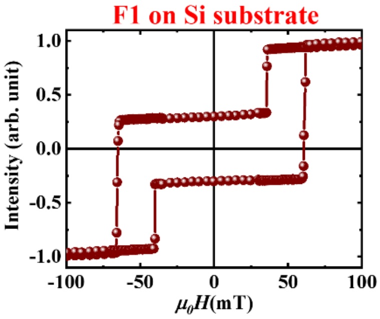


Figure S6: Hysteresis loop measured by MOKE microscopy for the Si counterpart of the flexible sample.

Figure S7 shows the domain images of the SAF sample prepared on PI substrate. The points (a), (b), (c) and (d) on the hysteresis loop represents the points at which domain images are taken for flat state as well as bend state (both concave and convex).

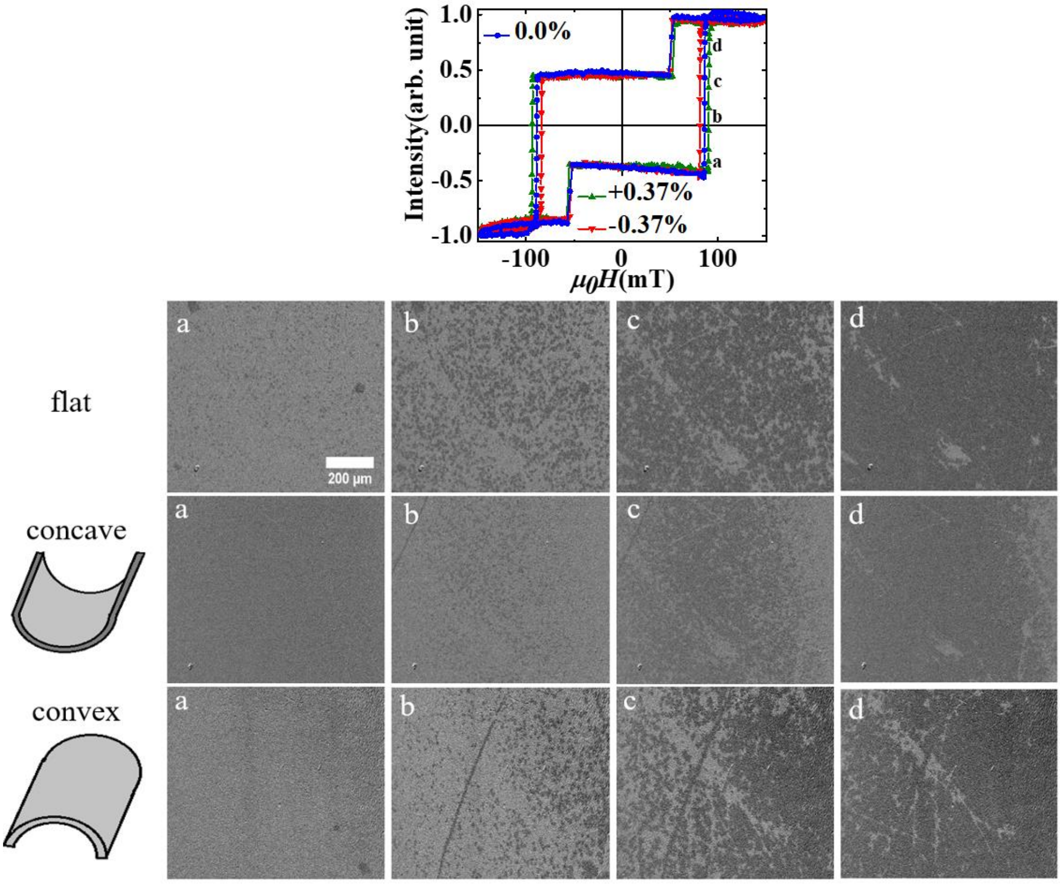


Figure S7: Domain images of sample F1 near reversal in flat state as well as bend state.
